# Supplementary material for: SonoEdit: Null-Space Constrained Knowledge Editing for Pronunciation Correction in LLM-Based TTS
Source: arXiv:2601.17086 source file (2026-01-23)
Supplement: Supplementary file 1 [file appendix.tex]

% \documentclass[11pt, a4paper]{article}

% % --- UNIVERSAL PREAMBLE BLOCK ---
% \usepackage[a4paper, top=2.5cm, bottom=2.5cm, left=2cm, right=2cm]{geometry}
% \usepackage{fontspec}
% \usepackage[english, bidi=basic, provide=*]{babel}
% \babelprovide[import, onchar=ids fonts]{english}
% \babelfont{rm}{Noto Sans}
% \babelfont{sf}{Noto Sans}
% \babelfont{tt}{Noto Sans Mono}
% % --------------------------------

% \usepackage{amsmath}
% \usepackage{amssymb}

% \title{Appendix: Implementation Details and Related Proofs}
% \author{}
% \date{}

% \begin{document}
% \maketitle

% \appendix

% Force the section counter to reset/start correctly for a standalone appendix document
\setcounter{section}{0}

\section{Implementation Details and Related Proofs}
\label{app:implementation_proofs}

In this section, we provide the detailed proofs regarding the null space properties and the derivation of the closed-form solution used in our methodology.

\subsection{Proof for the Shared Null Space of $K_0$ and $K_0 K_0^T$}
\label{app:null_space_proof}

\textbf{Theorem:} Let $K_0$ be a $m \times n$ matrix. Then $K_0$ and $K_0 K_0^T$ share the same left null space.

\textbf{Proof:}
Define the left null space of a matrix $A$ as the set of all vectors $\mathbf{x}$ such that $\mathbf{x}^T A = 0$. We need to show that if $\mathbf{x}$ is in the left null space of $K_0$, then $\mathbf{x}$ is also in the left null space of $K_0 K_0^T$, and vice versa.

\begin{enumerate}
    \item \textbf{Inclusion $\mathcal{N}\left(\mathbf{x}^T K_0\right) \subseteq \mathcal{N}\left(\mathbf{x}^T K_0 K_0^T\right)$:}
    \begin{itemize}
        \item Suppose $\mathbf{x}$ is in the left null space of $K_0$, \textit{i.e.}, $\mathbf{x}^T K_0 = \mathbf{0}$.
        \item It follows that $\mathbf{x}^T\left(K_0 K_0^T\right)=\left(\mathbf{x}^T K_0\right) K_0^T=\mathbf{0} \cdot K_0^T=\mathbf{0}$.
        \item Therefore, $\mathbf{x}$ is in the left null space of $K_0 K_0^T$.
    \end{itemize}

    \item \textbf{Inclusion $\mathcal{N}\left(\mathbf{x}^T K_0 K_0^T\right) \subseteq \mathcal{N}\left(\mathbf{x}^T K_0\right)$:}
    \begin{itemize}
        \item Suppose $\mathbf{x}$ is in the left null space of $K_0 K_0^T$, \textit{i.e.}, $\mathbf{x}^T\left(K_0 K_0^T\right)=\mathbf{0}$.
        \item Multiplying by $\mathbf{x}$ from the right, we get $\mathbf{x}^T K_0 K_0^T \mathbf{x} = 0$, which simplifies to $(\mathbf{x}^T K_0) (\mathbf{x}^T K_0)^T = \|\mathbf{x}^T K_0\|^2 = 0$.
        \item Since the norm is zero, the vector itself must be zero: $\mathbf{x}^T K_0 = \mathbf{0}$.
        \item Hence, $\mathbf{x}$ is also in the left null space of $K_0$.
    \end{itemize}
\end{enumerate}

From these arguments, we establish that both $K_0$ and $K_0 K_0^T$ share the same left null space. This equality allows us to compute the null-space projection using the lower-dimensional covariance matrix $K_0 K_0^T$ instead of the high-dimensional $K_0$.

\subsection{Proof for Equation $\Delta W P K_0 K_0^T = 0$}
\label{app:projection_proof}

Let the Singular Value Decomposition (SVD) of $K_0 K_0^T$ be given by eigenvectors $U$ and eigenvalues $\Sigma$. We can partition $U$ and $\Sigma$ as $U = [U_1, U_2]$ and $\Sigma = \text{diag}(\Sigma_1, \Sigma_2)$, where $\Sigma_2 \approx 0$ contains the zero (or near-zero) eigenvalues, and $U_2$ consists of the corresponding eigenvectors.

Since $U$ is an orthogonal matrix, it follows that:
\begin{equation}
U_2^T K_0 K_0^T = U_2^T U_1 \Sigma_1 U_1^T = \mathbf{0}.
\end{equation}

This implies that the column space of $U_2$ spans the null space of $K_0 K_0^T$. Accordingly, the projection matrix $P$ onto this null space is defined as:
\begin{equation}
    P = U_2 U_2^T.
\end{equation}

Consequently, for any update $\Delta W$ projected by $P$:
\begin{equation}
\Delta W P K_0 K_0^T = \Delta W U_2 U_2^T K_0 K_0^T = \mathbf{0},
\end{equation}
which confirms that applying $P$ ensures the update lies within the null space of the preserved knowledge.

\subsection{Derivation of the Update Rule}
\label{app:derivation}

We aim to minimize the objective function for the update $\Delta W$:
\begin{equation}
J = \|(W + \Delta \tilde{W} P) K_1 - V_1\|_F^2 + \|\Delta \tilde{W} P\|_F^2 + \|\Delta \tilde{W} P K_{prev}\|_F^2,
\end{equation}
where $K_{prev}$ represents keys from previous edits (if any) that must also be preserved. Let $R = V_1 - W K_1$ be the residual error. Setting the derivative $\frac{\partial J}{\partial \Delta \tilde{W}}$ to zero yields:
\begin{equation}
(\Delta W P K_1 - R) K_1^T P^T + \Delta W P P^T + \Delta W P K_{prev} K_{prev}^T P^T = \mathbf{0}.
\end{equation}

Utilizing the properties of the projection matrix ($P = P^T$ and $P^2 = P$), we can factorize $\Delta W P$:
\begin{equation}
\Delta W P \left( K_1 K_1^T P + I + K_{prev} K_{prev}^T P \right) = R K_1^T P.
\end{equation}

Right-multiplying by the inverse of the term in parentheses gives the closed-form solution:
\begin{equation}
\Delta W^* = \Delta W P = R K_1^T P \left( K_{prev} K_{prev}^T P + K_1 K_1^T P + I \right)^{-1}.
\end{equation}
This solution ensures that the update corrects the target association ($K_1 \to V_1$) while remaining orthogonal to the preserved knowledge space defined by $P$.

\subsection{Invertibility of the Regularized Term}
\label{app:invertibility}

To prove the invertibility of the matrix $M = (K_{prev} K_{prev}^T P + K_1 K_1^T P + I)$, note that $K K^T$ forms are positive semidefinite. The projection $P$ projects onto a subspace, preserving semidefiniteness.

The addition of the identity matrix $I$ (or $\lambda I$ in a generalized form where $\lambda > 0$) acts as a regularizer. It shifts all eigenvalues of the matrix sum by $+1$ (or $+\lambda$), ensuring that all eigenvalues are strictly positive. A matrix with strictly positive eigenvalues is positive definite and, therefore, invertible. Thus, the solution $\Delta W^*$ is numerically stable and well-defined.
